# Supplementary material for: Leveraging Experience in Lifelong Multi-Agent Pathfinding
Source: arXiv:2202.04382 source file (2022-05-16)
Supplement: Supplementary file 1 [file appendix.tex]

\begin{figure*}[th!]  % * make it all page width figure
\centering
    \centering
    \begin{subfigure}[t]{0.65\columnwidth}
        \centering
        %\raisebox{.25\textwidth}
        {%
        \includegraphics[width=0.75\linewidth]{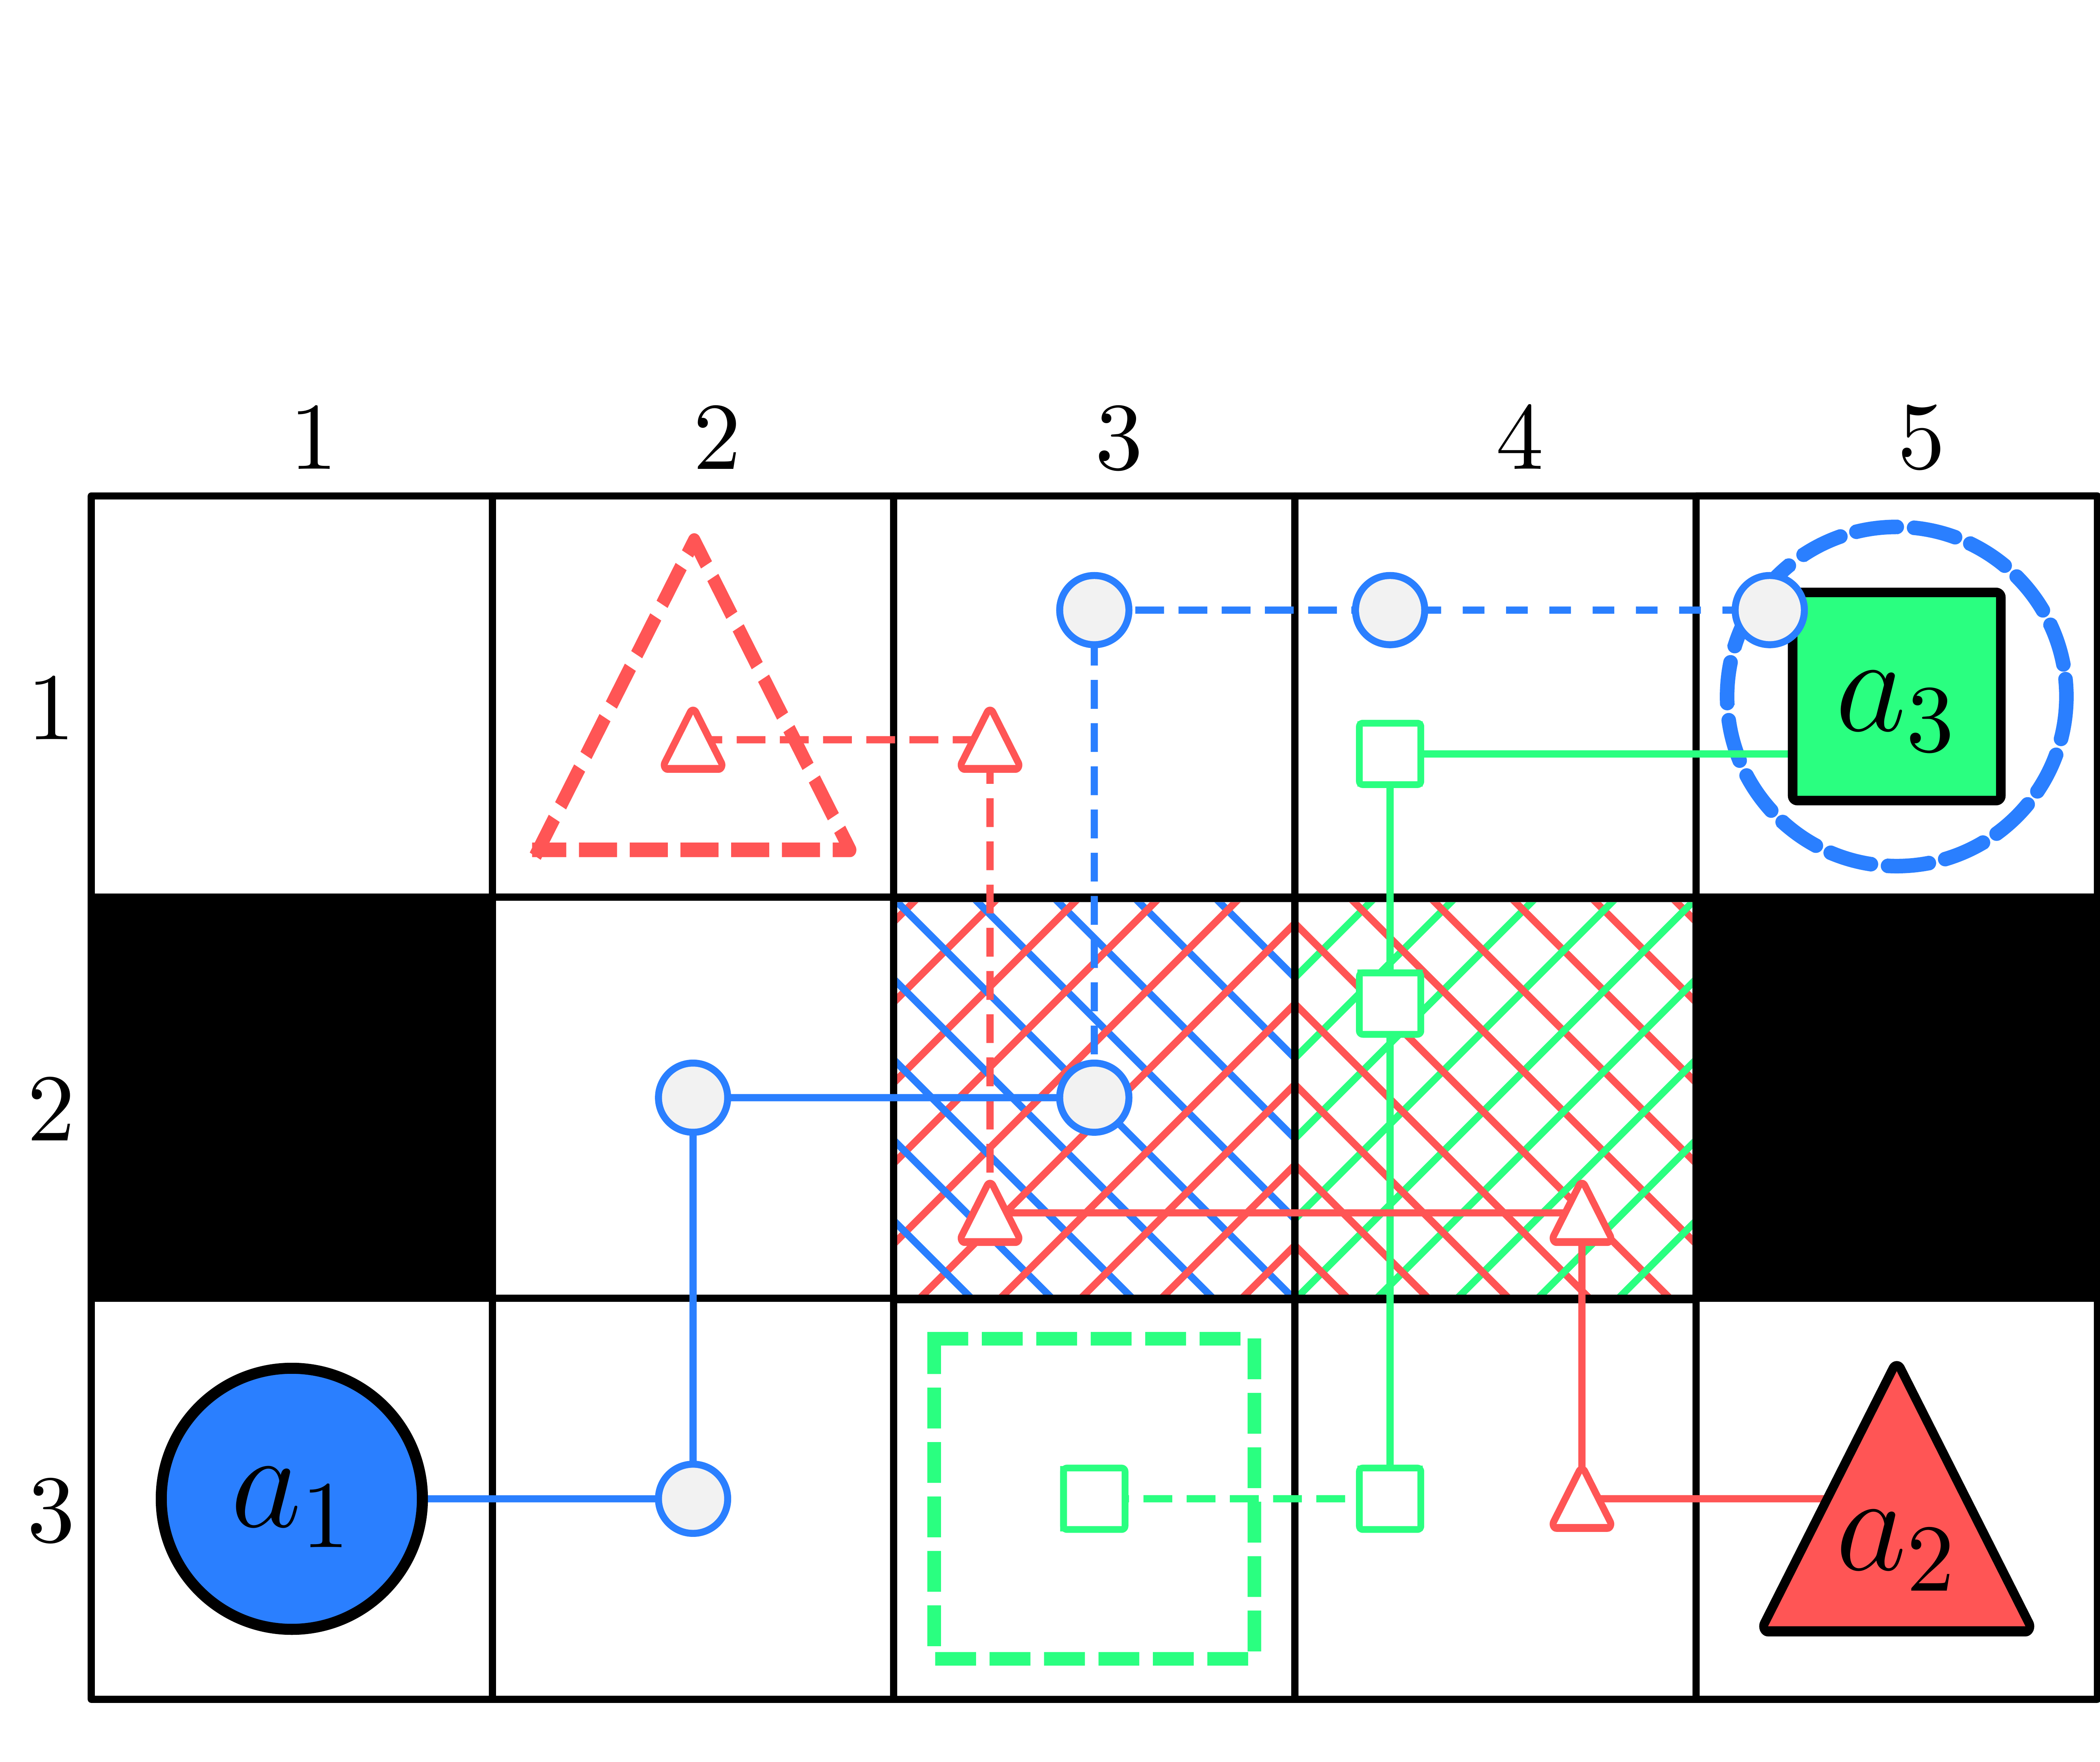} }
        \caption{Low-level search for the root node  $N_0$.} 
        \label{fig:toy_N0}
    \end{subfigure}
    \hfill
    \centering
    \begin{subfigure}[t]{0.65\columnwidth}
        \centering
        %\raisebox{.25\textwidth}
        {%
        \includegraphics[width=0.75\linewidth]{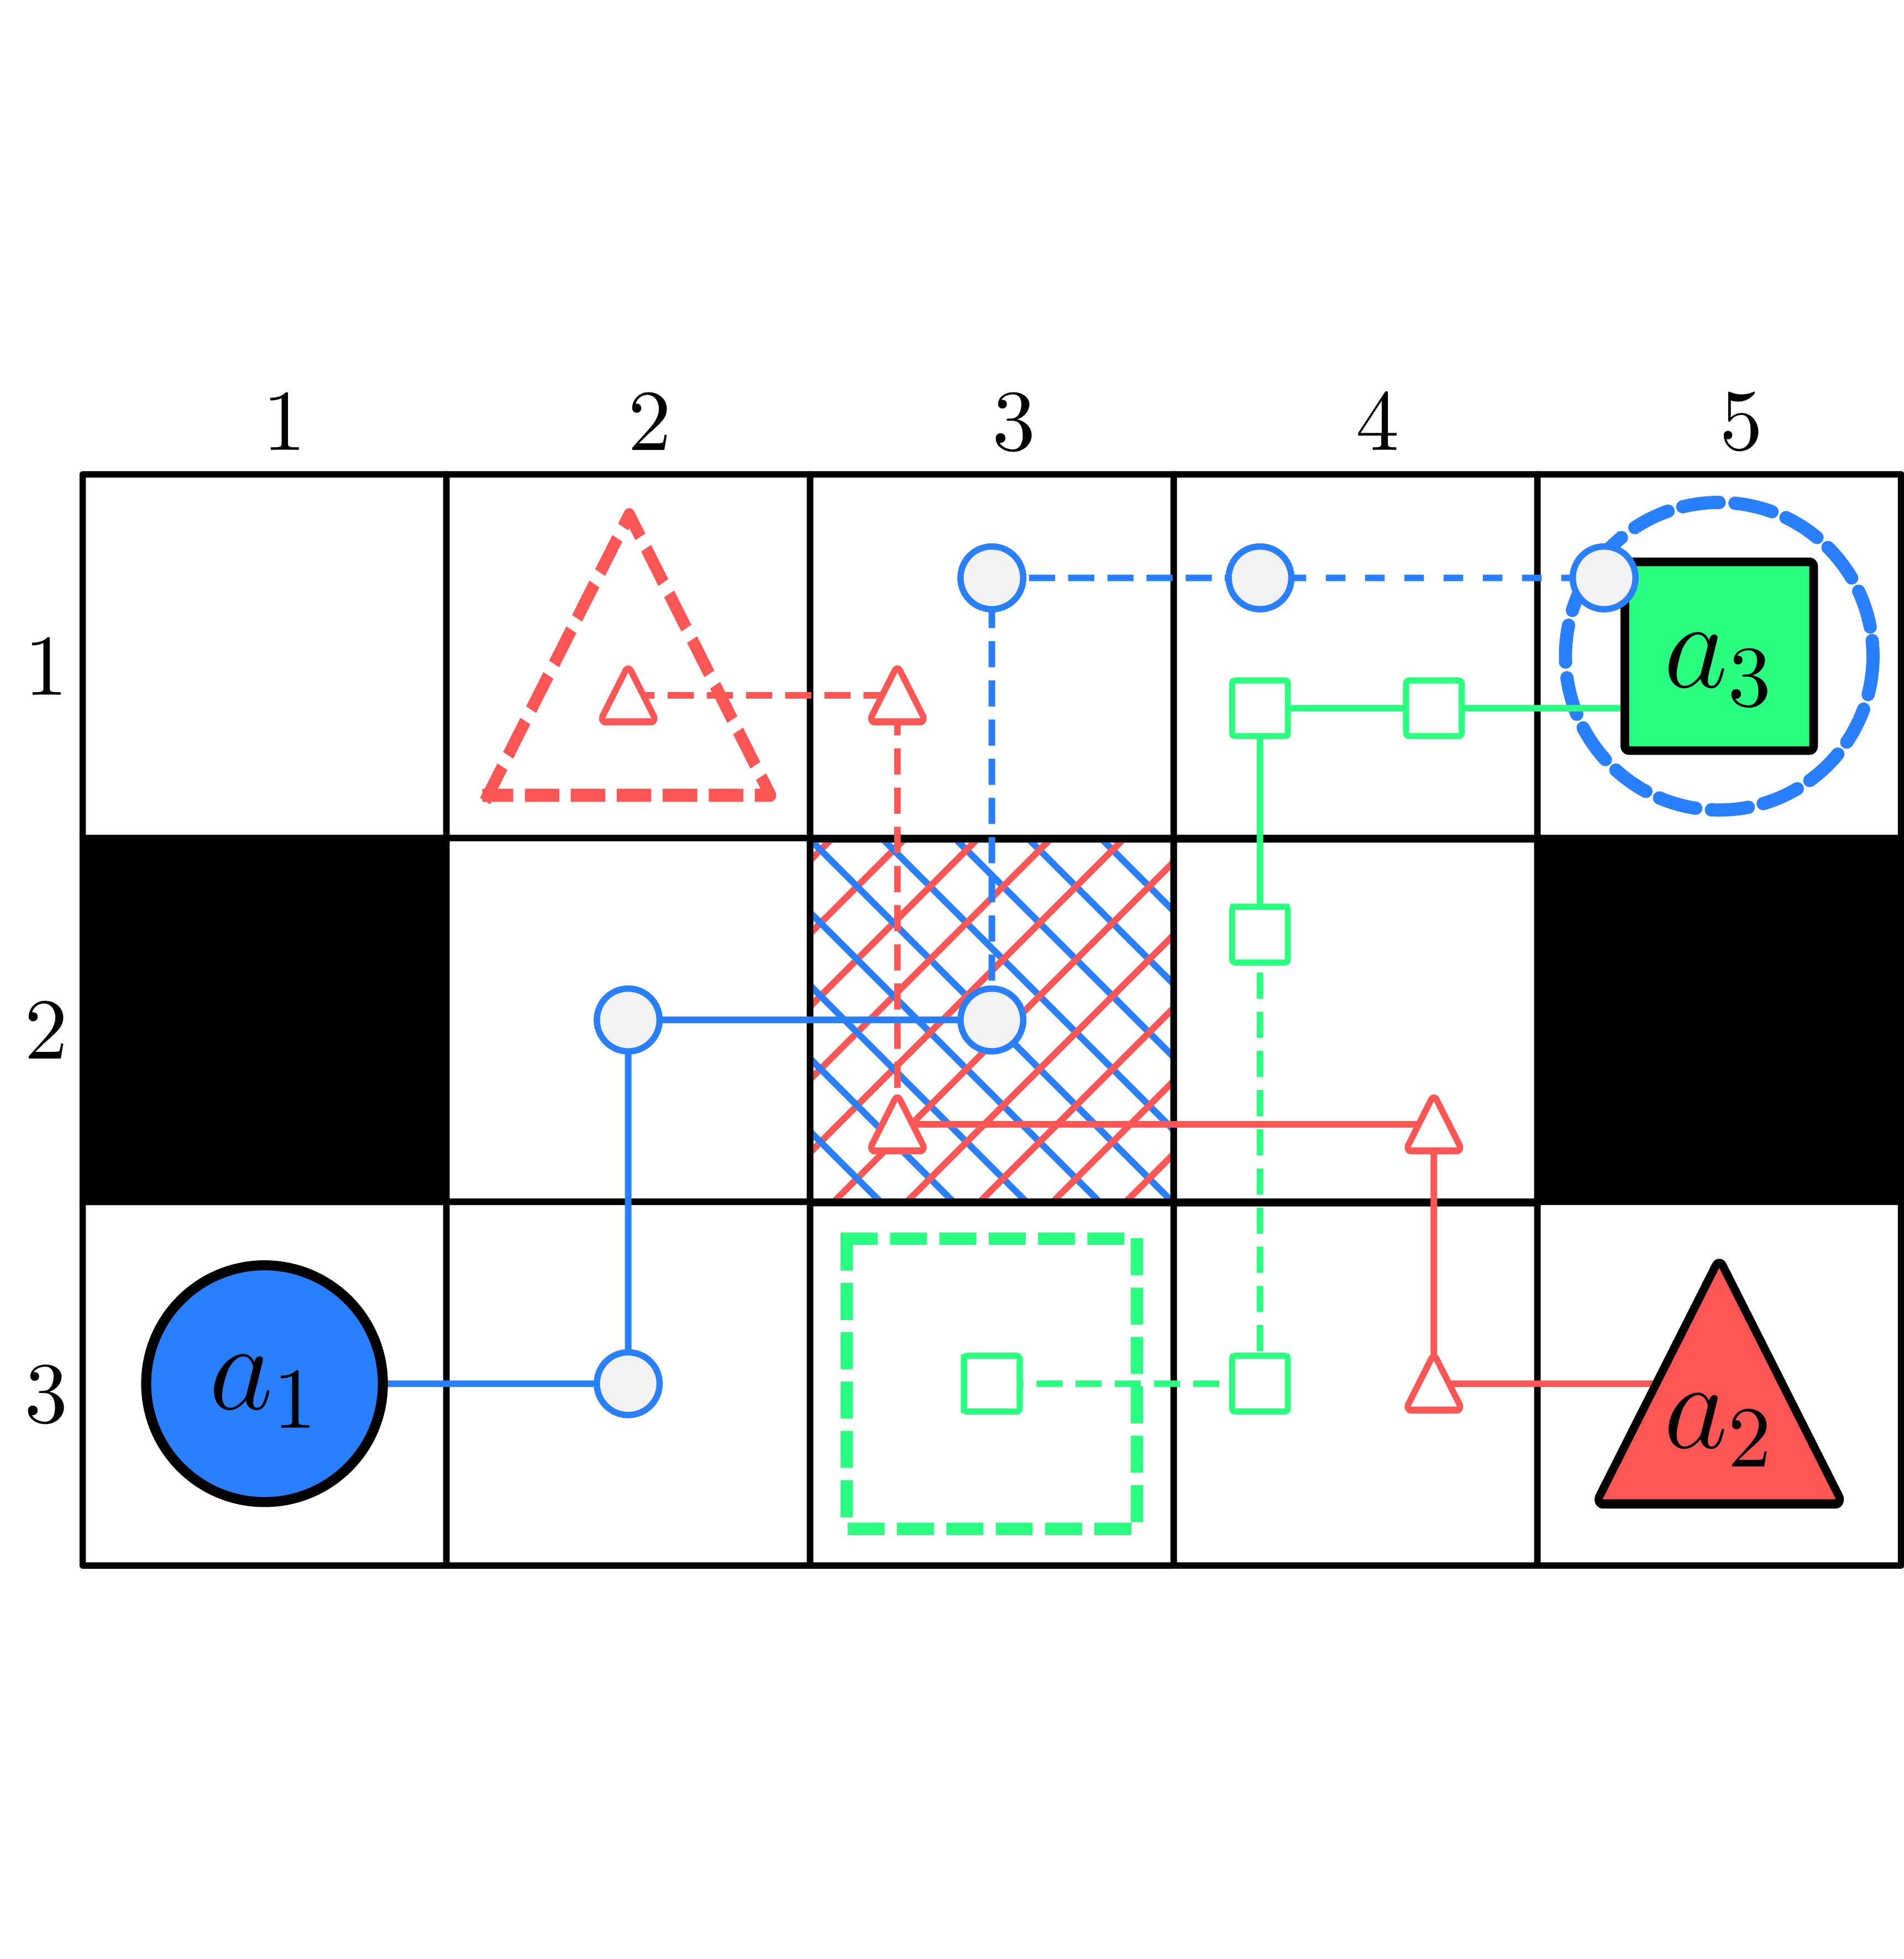} }
        \caption{Low-level search for the node $N_2$.} 
        \label{fig:toy_N2}
    \end{subfigure}
    \hfill
    \centering
    \begin{subfigure}[t]{0.65\columnwidth}
        \centering
        %\raisebox{.25\textwidth}
        {%
        \includegraphics[width=0.75\linewidth]{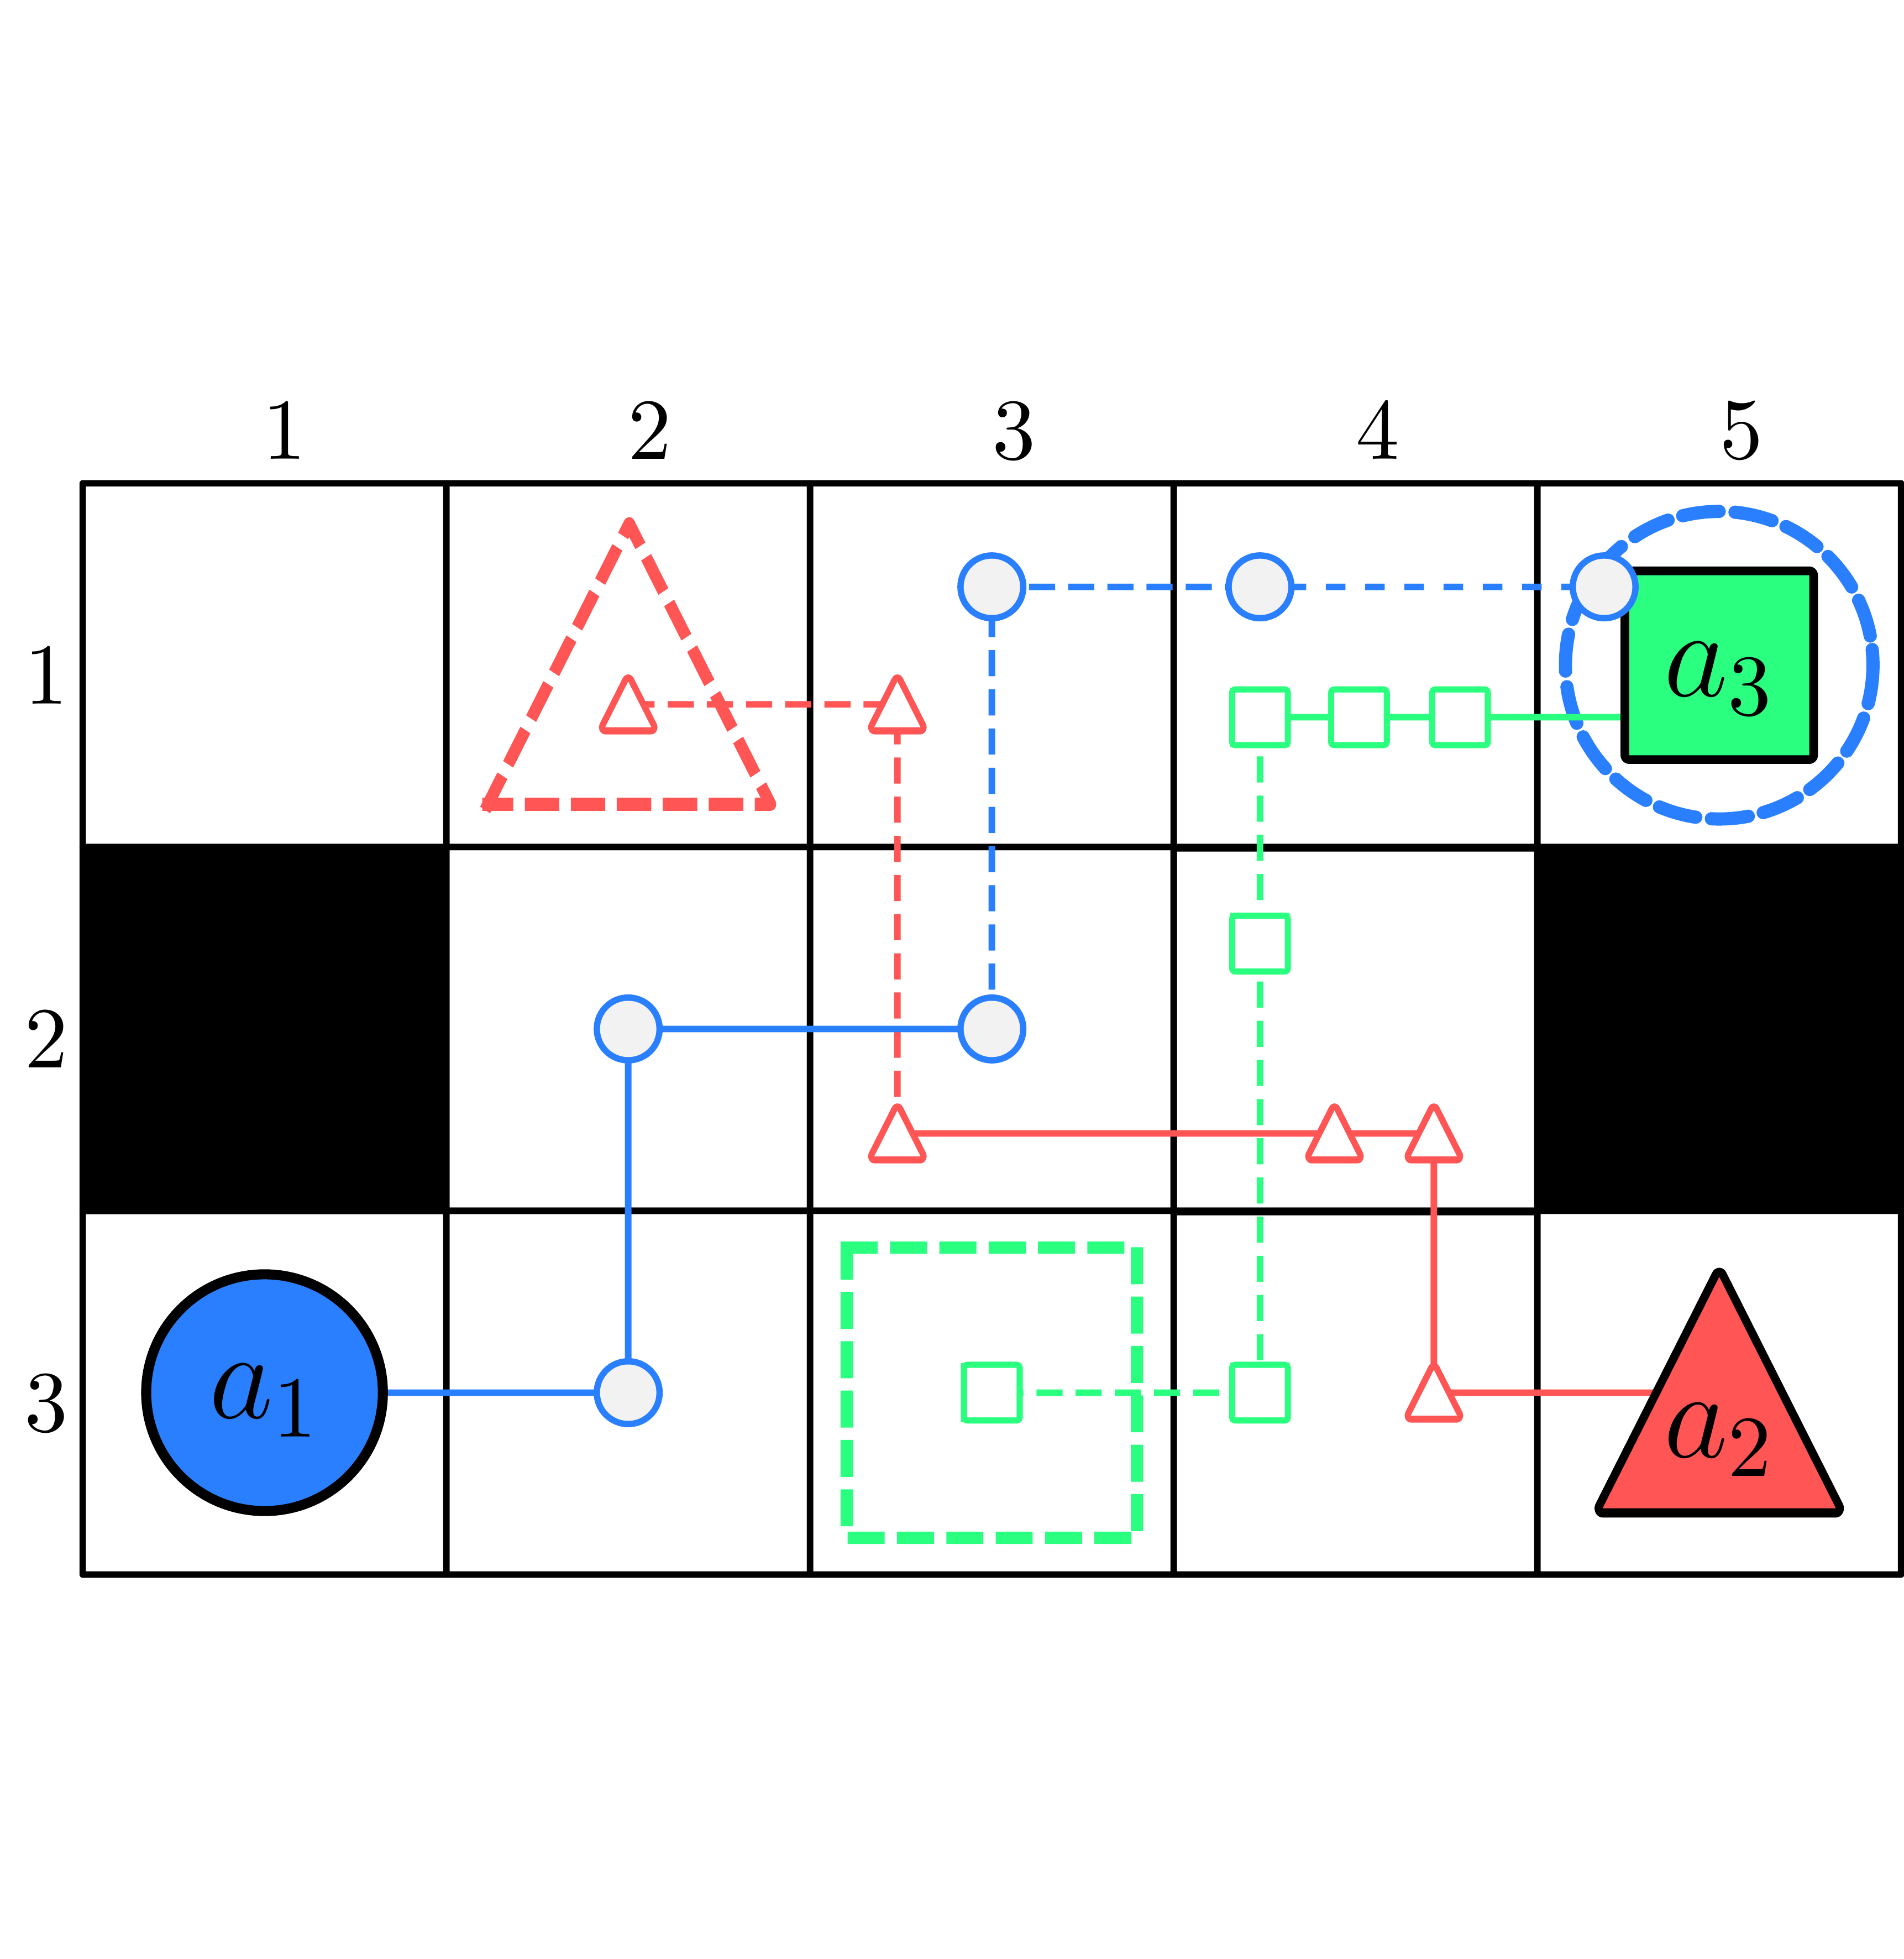} }
        \caption{Low-level search for the node $N_4$.} 
        \label{fig:toy_N4}
    \end{subfigure}
    \hfill
    \caption{Visualization of the low-level search of \pbs for W-MAPF query.}
\end{figure*}

\begin{figure}  % * make it all page width figure
    \vspace{-3mm}
    \centering
    \includegraphics[width=0.5\linewidth]{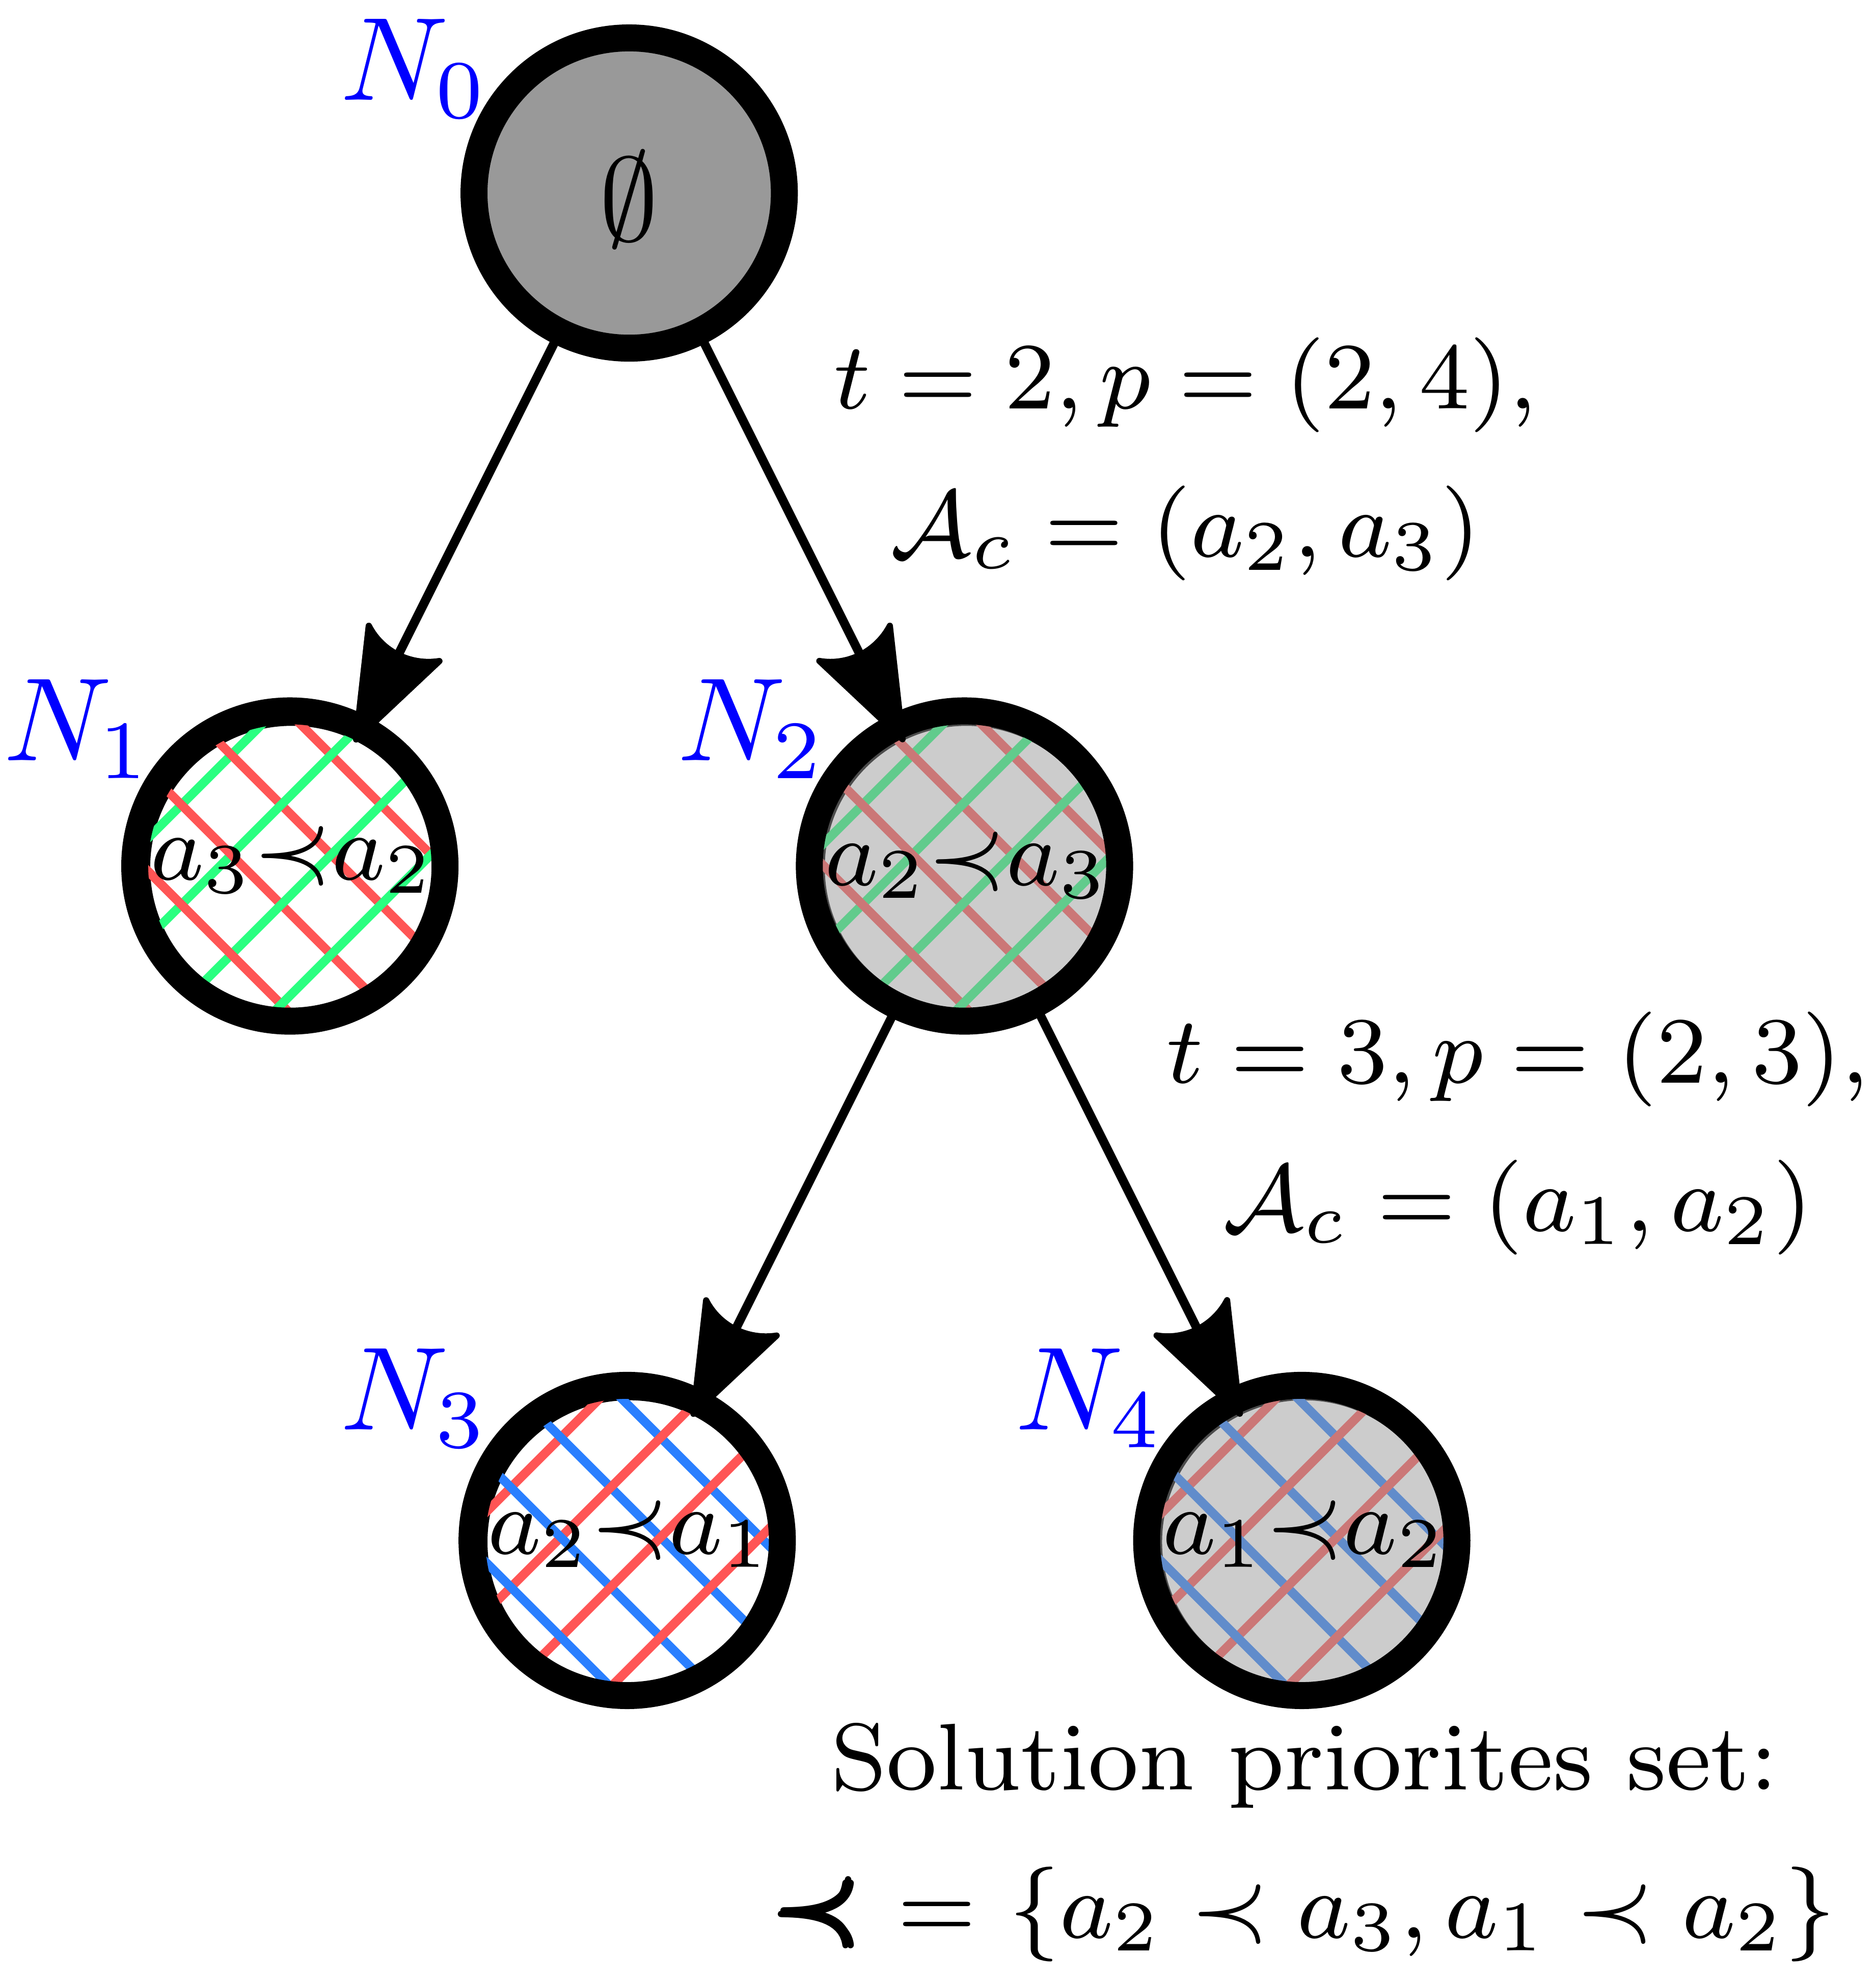} 
    \caption{\pbs search tree for W-MAPF query $q_0$.}
    \label{fig:toy_PT}
    \vspace{-7pt}
\end{figure}

\section*{Appendix}
\appendix
\NM{===== TODO - create a supplementary material document =====}
%In the \supplementary below 
We provide additional details and experiments that were omitted from the main text. We start (\Sec \ref{sec:toy}) by extending the explanation of the toy example (\Fig 2 of the main text) to also account for the behavior of \pbs while solving the first W-MAP query in the toy example.
We then continue (\Sec \ref{sec:add-exp}) to provide some additional results to illustrate the performance of \exrhcr beyond runtime.

\section{Additional Experimental Results}
\label{sec:add-exp}
We describe additional experimental results that were omitted from the main text. In particular, we give additional details on the throughput improvement achieved with \exrhcr (\Sec \ref{sec:ex:throughput}), the depth of the PT tree with \expbs (\Sec \ref{sec:depth}), and the impact of the width limit on the performance of \exrhcr (\Sec \ref{sec:wldfs}). 

\subsection{Maximal Throughput Comparison}\label{sec:ex:throughput}

% \begin{figure}[t]  % * make it all page width figure
%     \centering
%         \includegraphics[width=.99\linewidth]{graphics/best_throughput_compare.pdf} 

%     \caption{A box plot of the maximal throughput obtained for the scenarios described in \Sec 5 of the main text.}
%     \label{fig:box_plot}
% \end{figure}

In the main text we report the relative throughput improvement of \exrhcr in comparison to \rhcr given a time budgets ($30$ for \warehouse and $90$ for \sorting).  %between maximal throughput of \rhcr and \exrhcr, per instance.
Figure~\ref{fig:box_plot} shows a box plot with the throughput of \rhcr with $k_{\rhcr}$ agents, and for \exrhcr with $k_{\exrhcr}$ agents.

\begin{figure}[t!]  % * make it all page width figure
    \centering
    \begin{subfigure}[t]{0.49\columnwidth}
        \centering
        \includegraphics[width=\linewidth]{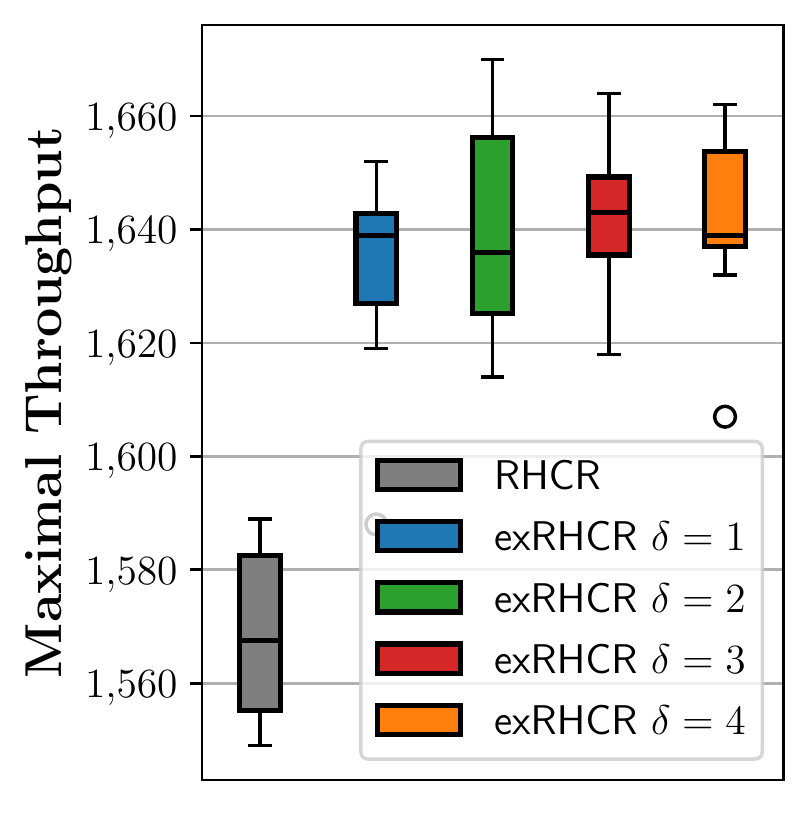} 
        \caption{Throughput for \warehouse.} 
        \label{fig:throughput_warehouse}
    \end{subfigure}
    \hfill
    \centering
    \begin{subfigure}[t]{0.49\columnwidth}
        \centering
        \includegraphics[width=\linewidth]{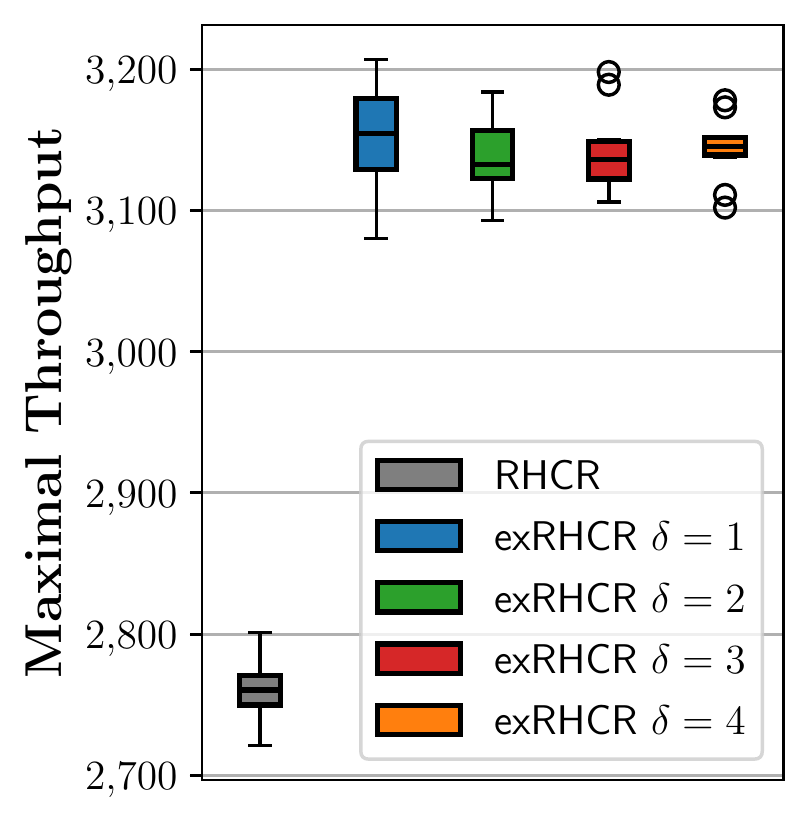} 
        \caption{Throughput for \sorting.} 
        \label{fig:throughput_sorting}
    \end{subfigure}
    \hfill
    \caption{A box plot of the maximal throughput obtained for the scenarios described in \Sec 5 of the main text.
    The number of agents~$k_{\rhcr}$ and $k_{\exrhcr}$ used by \rhcr and \exrhcr, respectively, are
    $k_{\rhcr}=140$ and $k_{\exrhcr}=150$ for \warehouse
    and~$k_{\rhcr}=300$ and $k_{\exrhcr}=350$ for \sorting.
    %In %\Fig 
    %\protect (\subref{fig:throughput_warehouse}) the number of agents used are: $k_{\rhcr}=130, k_{\exrhcr}=150$, and in %\Fig 
    %\protect (\subref{fig:throughput_sorting}) $k_{\rhcr}=300, k_{\exrhcr}=350$
    }
    \label{fig:box_plot_}
\end{figure}

\subsection{Effect of Width Limit with \wldfs}
\label{sec:wldfs}
Here we assess how the width limit parameter $\ell$ affects the performance of \expbs and consequently \exrhcr. Recall that this parameter limits the width of the PT tree, and causes \expbs to restart the search from \pbs with the empty PT root $\emptyset$ when the width constraint is violated. That is, we use \wldfs instead of \dfs within the PT high-level search. 

To test the affect of $\ell$ we generated $10$ L-MAPF instances for the \warehouse environment (as described in the main text) with the number of agents fixed on $k=160$, lookahead $\delta=3$, and report average metrics (detailed shortly) for MAPF queries for different values of $\ell \in \{2, 5, 10, 20, 50, 1{,}000\}$ in \Fig \ref{fig:wldfs_poc}. Note that for $\ell=2$ \expbs behaves very similarly to $\pbs$ as it immediately reverts to \pbs if the priority set in the root node leads to collisions. The setting of $\ell=1{,}000$ simulates a version wherein no fallback is taken and \expbs is essentially equivalent to \pbs. 

We have logged for every value of $\ell$ the following attributes that are averaged across all MAPF queries  (starting with the top attribute and going in a clockwise manner with respect to \Fig \ref{fig:wldfs_poc}): (i) average runtime; (ii) average PT width; (iii) average number of \astar node expansions in the low-level \expbs and \pbs search; (iv) average number of PT node expansions in the high-level \expbs and \pbs search; (v) average depth of PT. 
The reported values are normalized. 

%We now elaborate on the effect of $\ell$. 
Observe that having no opportunity to reuse experience ($\ell=2$), or allowing the search to explore the PT rooted in a seed experience indefinitely ($\ell=1{,}000$), significantly reduces the performance of \exrhcr in comparison with the other $\ell$ values for all attributes (i)--(v), which indicates that using \wldfs is indeed beneficial. \NM{TODO- add explanation that $l=2$ effect is "small damage w.h.p." and $\ell=1{,}000$ is "big damage w.l.p."}

% Figure~\ref{fig:wldfs_poc} demonstrate an experience we make to test \wldfs.
% We used the \warehouse domain with $k=160, \delta=3$ and $\ell \in \{2, 5, 10, 20, 50, 1{,}000\}$.
\begin{figure}[t!]  % * make it all page width figure
    \centering
    \includegraphics[width=\linewidth]{graphics/spyder_WLDFS_with_depth.pdf} % add with_depth at the end for extended plot
    \caption{A radar plot depicting the affect of the width limit $\ell$ on various attributes of \exrhcr. \NM{The values in each axis are normalized by the maximum value}}
    \label{fig:wldfs_poc_}
\end{figure}

\subsection{Average Solution  Depth Comparison} \label{sec:depth}
\begin{figure*}[t!]  
    \centering
    \begin{subfigure}[t]{0.99\columnwidth}
        \centering
        \includegraphics[width=\columnwidth]{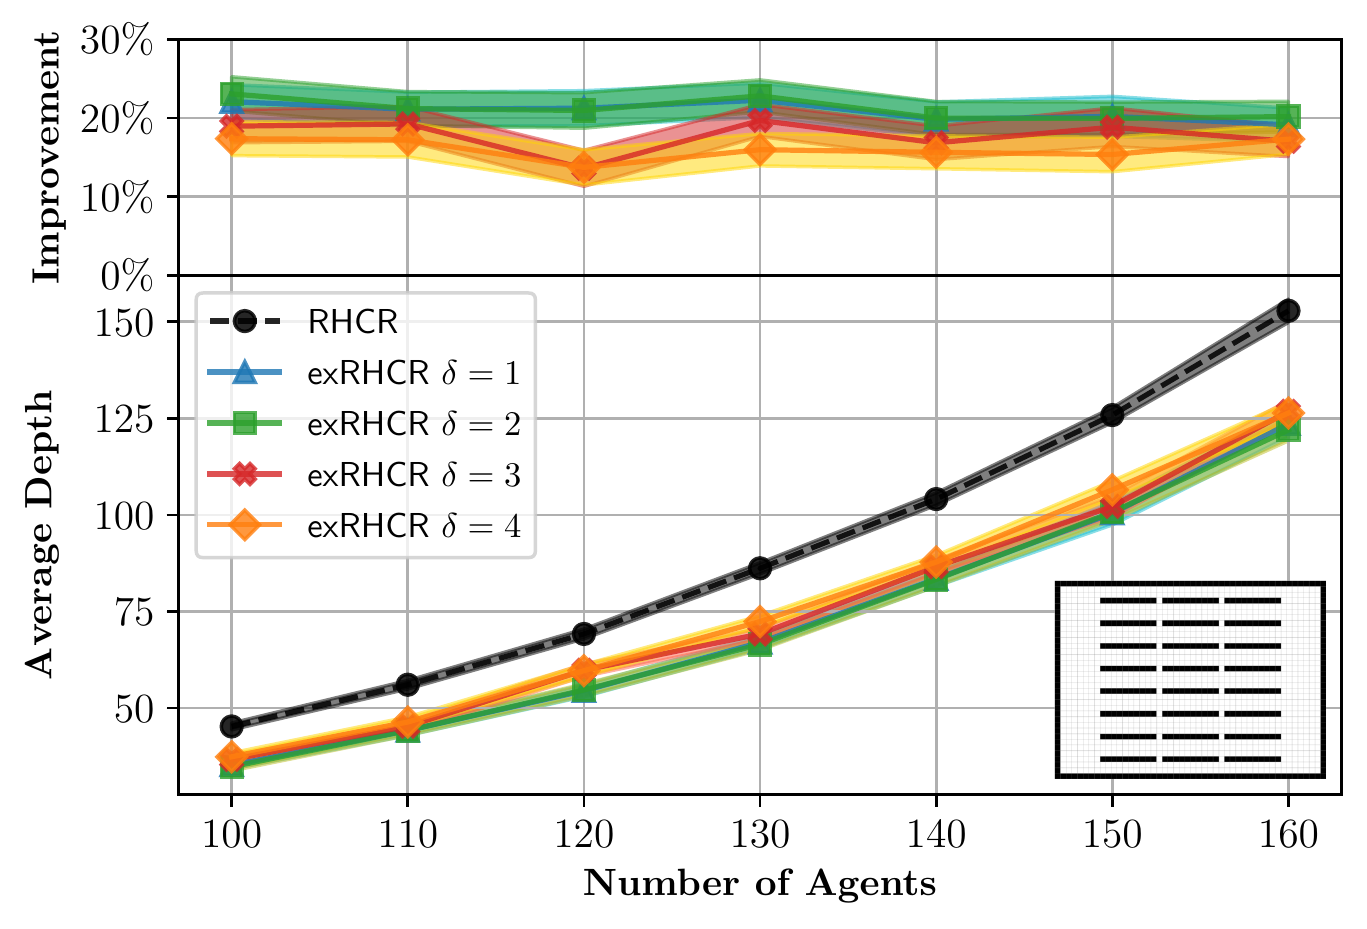}
        \caption{Solution depth for \warehouse.}
        \label{fig:lifelong_kiva_depth}
    \end{subfigure}
    \hfill
    \begin{subfigure}[t]{0.99\columnwidth}
        \centering
        \includegraphics[width=\columnwidth]{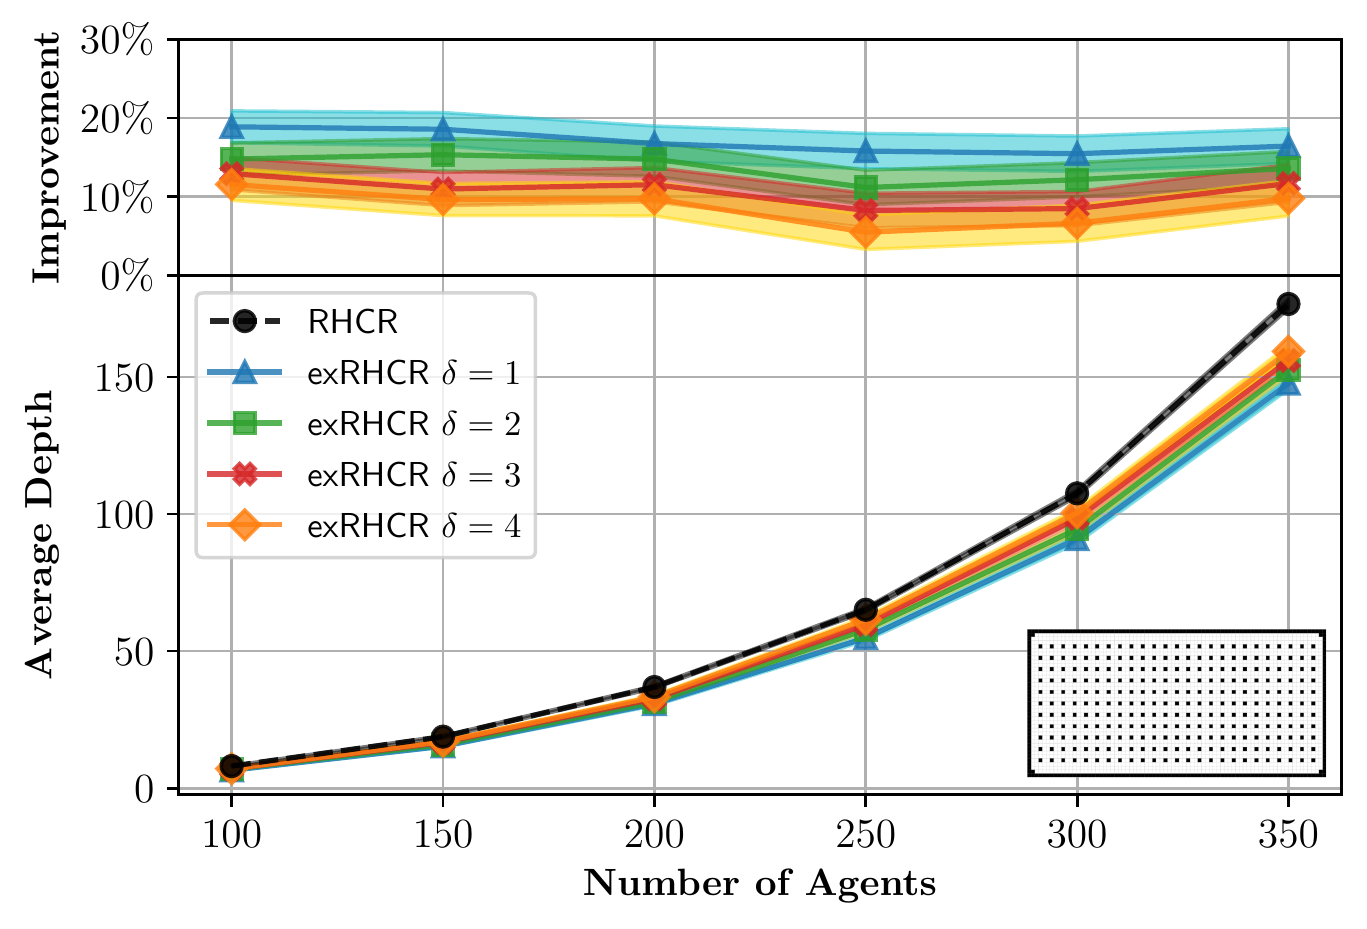} 
        \caption{Solution depth for \sorting.} 
        \label{fig:lifelong_sorting_depth}
    \end{subfigure}
    \caption{The average solution PT depth obtained for the scenarios described in \Sec 5 of the main text.}
    \label{fig:depth}
\end{figure*}

In addition to the runtime comparison we provided in the main paper, we provide here a similar comparison with respect to the depth of the solution PT node (\Fig \ref{fig:depth}). That is, we report the average depth of the node in which a solution is found across all MAPF instances, where we used the same L-MAPF instances as before. %In case of a fallback, the reported depth of a MAPF query is the sum between the depths of the PT of \expbs and \pbs.
Since the PT depth is highly correlated with solution time, we observe here as well that \exrhcr significantly improves upon \rhcr. There is however a difference in the standard deviation, which is smaller now. Interestingly, the percentage of improvement seems to be quite consistent across various numbers of agents $k$, which suggests that depth is  insensitive to $k$.  %constant which means the our framework reduces the PT size in similar manner and not depended on $k$.

\newpage

\section{Additional Details for Toy Example}
\label{sec:toy}

We now extend the explanation of the \exrhcr toy example we used in \Fig 2 of the main text by providing a visualization of how \pbs constructs its PT and obtains a  solution  for the first W-MAPF query $q_0$. As a reminder, the parameter used are: $w=4, h=2, \delta=2$ and we have three agents (solid shapes) with three assigned tasks represented by goal location in dashed shapes. 

In \Fig \ref{fig:toy_PT} we visualize the final structure of the PT tree of \pbs after a solution is found. The high-level search begins in the root node~$N_0$ with the empty priority set. \Fig \ref{fig:toy_N0} illustrates the solution paths obtained by the low-level search for node~$N_0$. In particular, each agent takes its shortest path without regard to the other agents as no priorities were specified. 
The paths are:
\begin{equation*} \label{eq1}
\begin{split}
\calP   = \{ &
p_{a_1}: [(3, 1), (3, 2), (2, 2), (2, 3), (1, 3), (1, 4), (1, 5) ], \\
 & p_{a_2}: [ (3, 5), (3, 4), (2, 4), (2, 3), (1, 3), (1, 2) ], \\
 & p_{a_3}: [ (1, 5), (1, 4), (2, 4), (3, 4), (3, 3) ]  
 \}
\end{split}
\end{equation*}
where for a pair $(\cdot, \cdot)$ the values represent the row and column numbers of a cell. As shown, the first collision $\calA_c=(a_2, a_3)$ occurs between agent $a_2$ and agent $a_3$, at timestep $t=2$ in position $p=(2, 4)$ (this position is visualized with a criss-cross red-green pattern denoting the agents in collision).
The second collision occurs between agent $a_1$ and $a_2$ at timestep $t=3$ in position $p=(2, 4)$ (marked by blue-red criss-cross). Due to the collision, the node $N_0$ is expanded into the two nodes $N_0$ and $N_1$. As the first collision occurs between $a_2$ and $a_3$, the priority $a_3\prec a_2$ is added to the priority set of $N_1$, and $a_2\prec a_3$ to $N_2$. Note the internal node label denotes the added priority from the priority set of the parent node. 

Next, we assume for the purpose of the example that \dfs chooses $N_2$ for expansion (expanded nodes are marked with  gray background) and executes the low-level search to find paths that abide to the priority set $\PREC_{N_2}=\{a_2\prec a_3\}$. As there are no specified priorities between $a_1$ and~$a_2$ their paths from~$N_0$ remain as-is, whereas the path of agent $a_3$ is updated and a wait action is added at position $p=(1, 4)$, as it needs to be executed while giving precedence to $a_2$ (see \Fig \ref{fig:toy_N2}). The new path of $a_3$ is $p_{a_3} = [(1, 5), (1, 4), (1, 4), (2, 4),(3, 4),(3, 3)]$.
The current state search is still a conflict between $\calA_c=(a_1, a_2)$ as detailed before.
Consequently, two child nodes $N_3$ and $N_4$ with the additional priorities $a_2\prec a_1$ and $a_1\prec a_2$, respectively, are added to the PT.

In the next step of the high-level search, \dfs picks $N_4$ for expansion, where $\PREC_{N_4} = \{a_2 \prec a_3, a_1 \prec a_2 \}$, which induces the total priority order of $a_1 \prec a_2 \prec a_3$.
Correspondingly, a low-level solution can be defined to be
\begin{equation*} \label{eq2}
\begin{split}
\calP   = \{ &
p_{a_1}: [(3, 1), (3, 2), (2, 2), (2, 3), (1, 3), (1, 4), (1, 5) ], \\
 & p_{a_2}: [ (3, 5), (3, 4),(2, 4), (2, 4), (2, 3), (1, 3), (1, 2) ], \\
 & p_{a_3}: [ (1, 5), (1, 4),(1, 4), (1, 4), (2, 4), (3, 4), (3, 3) ]
 \}.
\end{split}
\end{equation*}
As there are no conflicts for the first  $w$ timesteps, we have a found a feasible solution (\Fig \ref{fig:toy_N4}).
Note that this solution is not unique:  other priorities set can be used to solve this W-MAPF, and different paths can be obtained by the low-level search depending on tie breaks.  %This solution is demonstrate the path updates by wait action to make this figure as clear as possible and simple.

% Figure~\ref{fig:toy_1} shows the \pbs solution, solid lines represent the paths calculated within the $w$ first timesteps, where collision is solved and dashed line represent the rest until reaching the goal, while ignoring other collisions. 
% Solid markers on the path lines represent the first $h$ steps and rest represented by hollow markers.

% Figure~\ref{fig:toy_2} represent the next W-MAPF sub-query. Here, the same collision needs to be solved, and assuming the expanded PT is similar (up to $h$ timesteps shift), \rhcr expand another two PT nodes.
% In contrast, \exrhcr will be executed with $\PREC_{\text{exp}}$ from the previous solution and thus will have a priority ordering set which solve those conflicts as input.
% Therefore, \exrhcr will expand no PT nodes (two nodes expansion is reduces).
% This explained our insight of reducing the PT size by leveraging experience. Moreover, it also demostrated here how our formulation of experience is generalizable despite the differences between the queries.

% Figure~\ref{fig:toy_3} shows the third W-MAPF sub-query, which have no conflict and therefore \rhcr will not expand PT node. \exrhcr, which still uses $\PREC_{\text{exp}}$ as a priorities seed, will also find path without conflict. This shows how our framework is robust for inappropriate experience information. Figure~\ref{fig:toy_4_solution} shows the terminal states where agents reached their goals and all tasks are done.

\begin{figure*}[t!]  % * make it all page width figure
\centering
    \begin{subfigure}[t]{1.95\columnwidth}
        \centering
        \vspace{5pt}
        \includegraphics[width=0.4\linewidth]{graphics/exRHCR_toy_example_PBS_PT.pdf} 
        \caption{\pbs search tree for W-MAPF query $q_0$.} 
        \label{fig:toy_PT}
    \end{subfigure}
    \hfill
    \centering
    \begin{subfigure}[t]{0.65\columnwidth}
        \centering
        %\raisebox{.25\textwidth}
        {%
        \includegraphics[width=\linewidth]{graphics/exRHCR_toy_example_PBS_N0.pdf} }
        \caption{Low-level search for the root node  $N_0$.} 
        \label{fig:toy_N0}
    \end{subfigure}
    \hfill
    \centering
    \begin{subfigure}[t]{0.65\columnwidth}
        \centering
        %\raisebox{.25\textwidth}
        {%
        \includegraphics[width=\linewidth]{graphics/exRHCR_toy_example_PBS_N2.pdf} }
        \caption{Low-level search for the node $N_2$.} 
        \label{fig:toy_N2}
    \end{subfigure}
    \hfill
    \centering
    \begin{subfigure}[t]{0.65\columnwidth}
        \centering
        %\raisebox{.25\textwidth}
        {%
        \includegraphics[width=\linewidth]{graphics/exRHCR_toy_example_PBS_N4.pdf} }
        \caption{Low-level search for the node $N_4$.} 
        \label{fig:toy_N4}
    \end{subfigure}
    \hfill
    % \centering
    % \begin{subfigure}[t]{0.65\columnwidth}
    %     \centering
    %     %\raisebox{.25\textwidth}
    %     {%
    %     \includegraphics[width=\linewidth]{graphics/exRHCR_toy_example_1.pdf} }
    %     \caption{Low-level search for the node $N_4$.} 
    %     \label{fig:toy_N4}
    % \end{subfigure}
    % \hfill
    
    % \begin{subfigure}[t]{0.65\columnwidth}
    %     \centering
    %     \includegraphics[width=\linewidth]{graphics/exRHCR_toy_example_2.pdf} 
    %     \caption{}
    %     \label{fig:toy_2}
    % \end{subfigure}
    % \hfill
    % \begin{subfigure}[t]{0.65\columnwidth}
    %     \centering
    %     \includegraphics[width=\linewidth]{graphics/exRHCR_toy_example_3.pdf} 
    %     \caption{} 
    %     \label{fig:toy_3}
    % \end{subfigure}
    % \hfill
    % \begin{subfigure}[t]{0.65\columnwidth}
    %     \centering
    %     \includegraphics[width=\linewidth]{graphics/exRHCR_toy_example_4_solution.pdf} 
    %     \caption{}
    %     \label{fig:toy_4_solution}
    % \end{subfigure}

    % \caption{An example of \exrhcr and \rhcr execution.}
    % \label{fig:toy_example}
    \caption{Visualization of (a)~the high-level and (b,c,d)~the low-level search of \pbs on the W-MAPF query $q_0$ from the toy example.}
\end{figure*}

\begin{figure}[t]  % * make it all page width figure
    \centering
    \begin{subfigure}[t]{0.24\columnwidth}
        \centering
        \includegraphics[width=\linewidth]{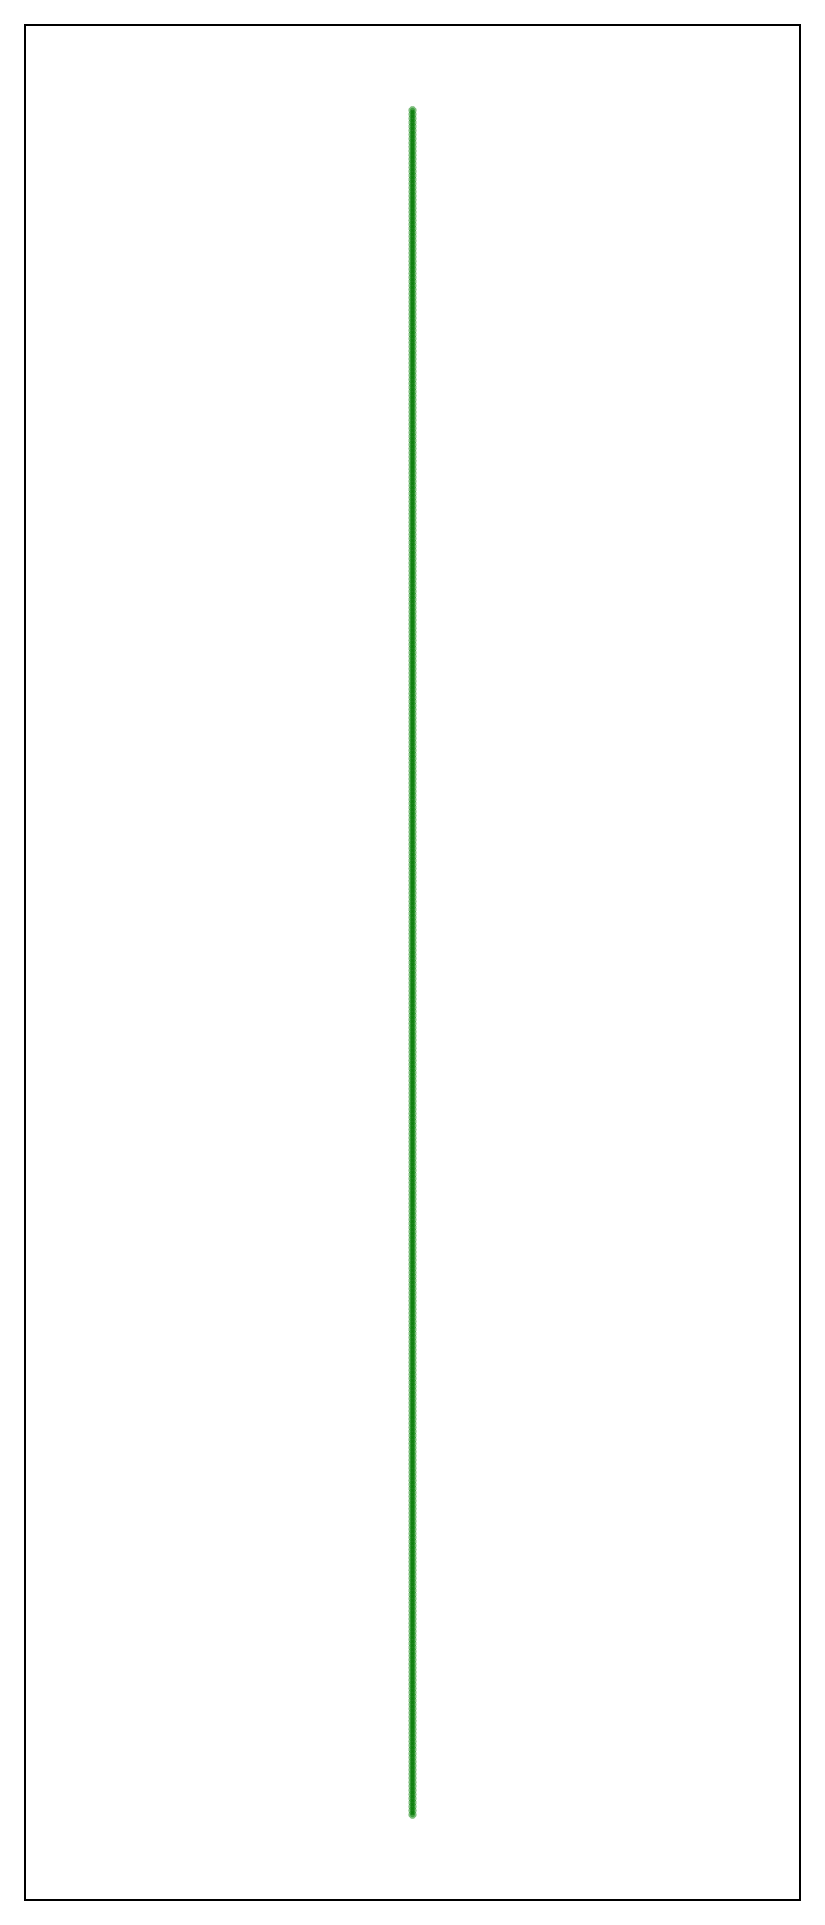} 
        \caption{} 
        \label{fig:hl_good_1_}
    \end{subfigure}
    \hfill
    \begin{subfigure}[t]{0.24\columnwidth}
        \centering
        \includegraphics[width=\linewidth]{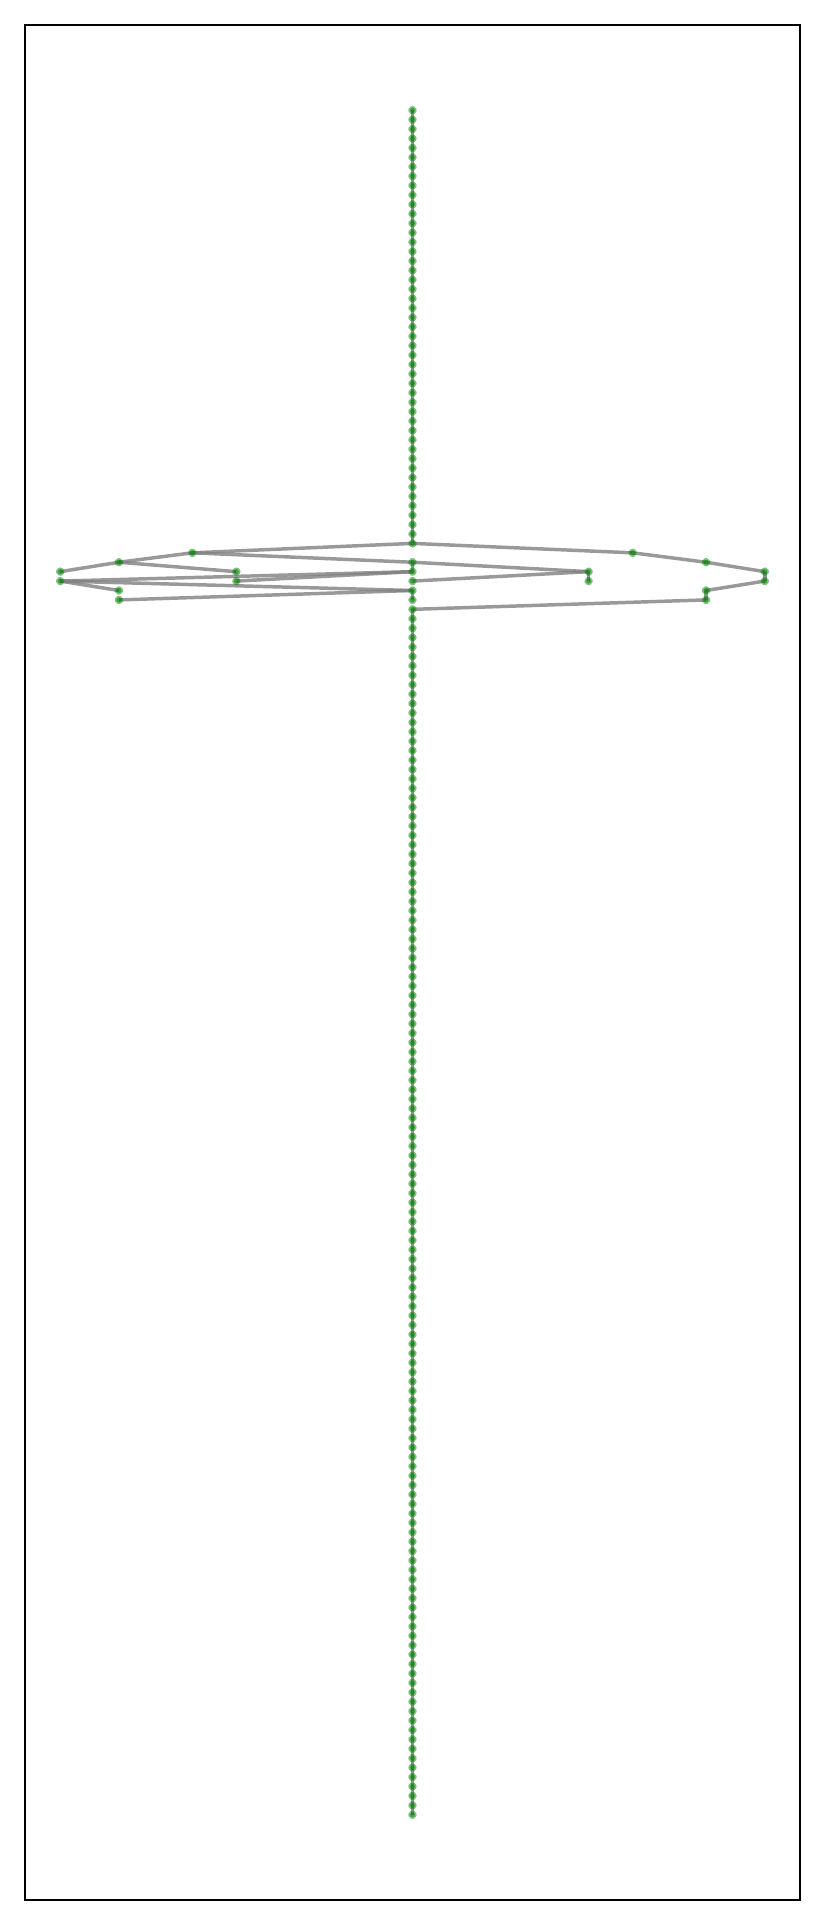} 
        \caption{}
        \label{fig:hl_good_2_}
    \end{subfigure}
    \hfill
    \begin{subfigure}[t]{0.24\columnwidth}
        \centering
        \includegraphics[width=\linewidth]{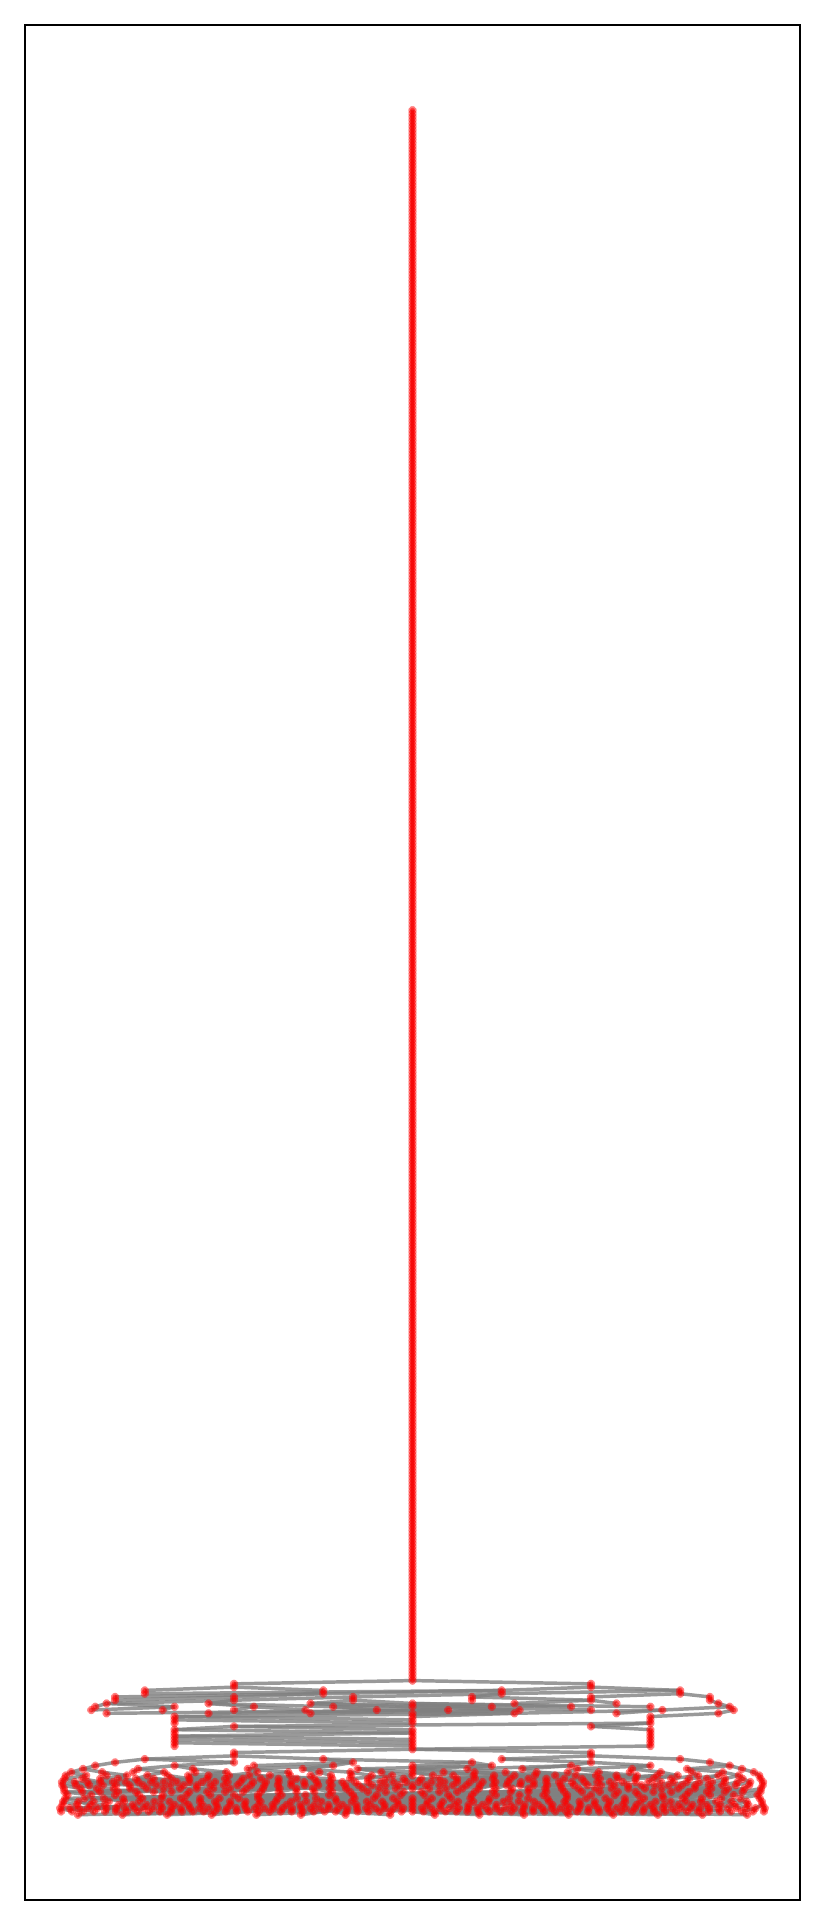} 
        \caption{} 
        \label{fig:hl_bad_1_}
    \end{subfigure}
    \hfill
    \begin{subfigure}[t]{0.24\columnwidth}
        \centering
        \includegraphics[width=\linewidth]{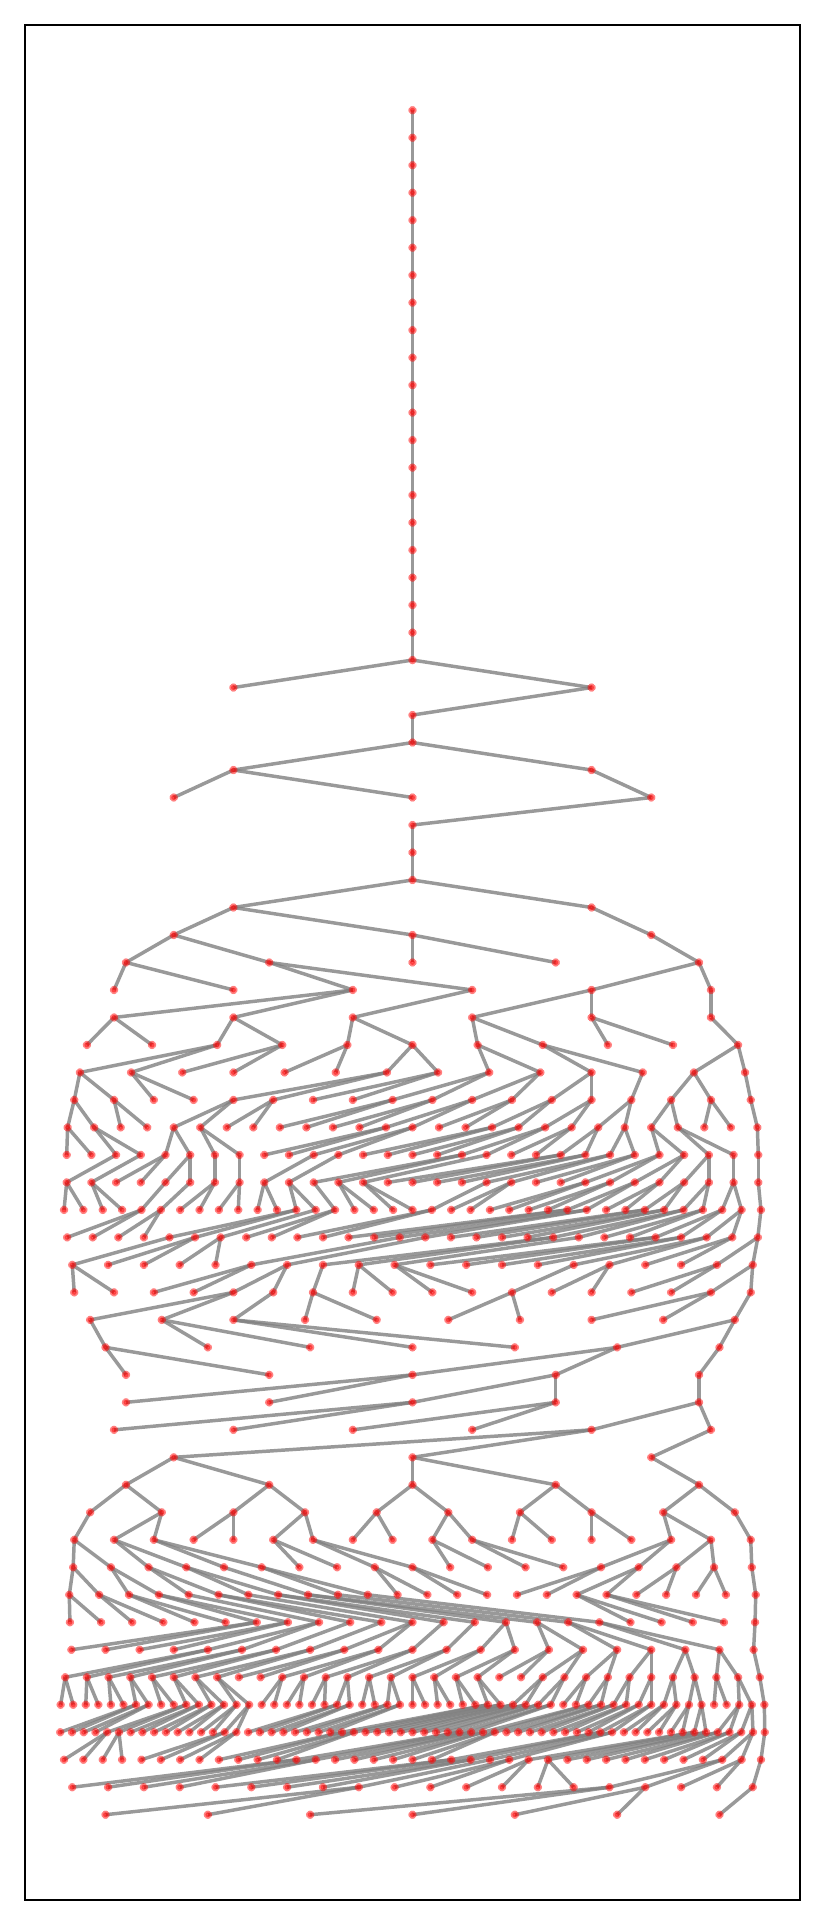} 
        \caption{}
        \label{fig:hl_bad_2_}
    \end{subfigure}

    \caption{Visualizations of \pbs expanded PTs using \dfs. 
    (a) and (b) in green demonstrates a search of resolved queries, 
    in (a) it resolved without backtracking in the \dfs tree 
    while in (b) the \dfs  search backtrack from some nodes during the process and found a solution after that. 
    (c) and (d) in red shows expanded \dfs trees of \pbs high-level for two unresolved queries due to runtime limit. 
    (c) demonstrate a short and wide \quot{dead-end} sub-tree 
    and (d) shows a tall and narrow one. 
    The common structure is that the search first expand node without backtracking. 
    We use this structure to manipulate the \dfs search in \expbs.
    \NM{rephrase caption + use it when explaining \wldfs }}
    \label{fig:dfs_hl_visualizations_}
\end{figure}
